# Supplementary material for: Nanodiamond quantum thermometry assisted with machine learning
Source: arXiv:2504.07582 source file (2025-04-10)
Supplement: Supplementary file 1 [file Supplementary_arXiv.pdf]

# Supplementary material: Nanodiamond quantum thermometry assisted with machine learning

Kouki Yamamoto*[1], Kensuke Ogawa[1], Moeta Tsukamoto[1], Yuto Ashida[1,2], Kento Sasaki[1], and Kensuke Kobayashi[1,2,3]

[1]Department of Physics, The University of Tokyo, Bunkyo-ku,Tokyo 113-0033, Japan
[2]Insititute for Physics of Intelligence, The University of Tokyo, Bunkyo-ku, Tokyo 113-0033, Japan
[3]Trans-Scale Quantum Scinece Institute, The University of Tokyo, Bunkyo-ku, Tokyo 113-0033, Japan

April 10, 2025

This is the Accepted Manuscript version of the Supplementary Material accompanying an article accepted for publication in *Applied Physics Express*. IOP Publishing Ltd is not responsible for any errors or omissions in this version of the supplementary material. This Supplementary Material is published under a CC BY licence. The Version of Record of the main article is available online at https://doi.org/10.35848/1882-0786/adac2a.

## Experimental setup

A laser beam (515 nm, 100 mW) is output through a multimode fiber and a collimator into the free space. A lens pair expands it before entering the objective lens (Mitsutoyo, M-PLAN APO 50X, numerical aperture NA=0.55, magnification ×50). The laser is focused by the objective lens and injected into the NDs (Adámas Nanotechnologies, NDNV100nmHi10ml) in the cryostat (Montana Instruments, Cryostation s-50) with temperature stability better than 10 mK. The top of the cryostat is equipped with an optical window through which the laser and the fluorescence from the NV centers pass. The fluorescence is then captured by a CMOS camera (Basler, acA2040-120um) after passing through the objective lens, a dichroic mirror, a 514 nm notch filter, a 650 nm long-pass filter, an 800 nm short-pass filter, and a 100 mm focal length imaging lens. The field of view size is about 280 $\mu$m×200 $\mu$m.

The resonator microwave antenna is placed directly above the optical window. The microwave antenna has a hole with a diameter of 2 mm, through which optical measurements are performed. The ODMR measurements are performed by inputting 25 dBm microwave power to the antenna. When acquiring the ODMR spectra, the microwave frequency is randomly swept at 321 equally spaced points from 2830 MHz to 2910 MHz, and this single frequency sweep is performed for about 45 seconds.

## Sample preparation

NDs are dispersed in water and dropped onto a copper plate with a thickness of 100 $\mu$m. They are spread using a spin coater at 500 revolutions per minute [1]. There are several to dozens of ND layers

*Corresponding author : kouki.yamamoto@phys.s.u-tokyo.ac.jp

using a spin coater under this condition. For example, the density of four ND layers would be about 1500 NDs/$\mu$m$^2$ [2]. The thickness of ND layers is not essential in this study.

# 4-point method

Conventional temperature analysis methods estimate the ZFS from ODMR spectra and convert the ZFS to temperature based on Eq. (1) in the main text. The basic idea of the widely used 4-point method is shown in Fig. 1(c) in the main text. Four frequency points in the ODMR spectrum are selected, and the changes in the ZFS are calculated from these values. As shown in Fig. 1(c) in the main text, the two points whose frequencies differ by $\delta f$ are selected from the left side slope of the lower dip in the spectrum, and the other two points are chosen from the right side slope of the larger dip similarly (i.e., four points are selected in total, such that $f_1$, $f_2$, $f_3$, and $f_4$ ($f_1 < f_2 < f_3 < f_4$), and $\delta f = f_2 - f_1 = f_4 - f_3$). Let $I_i$ ($i \in \{1, 2, 3, 4\}$) be the PL intensity at $f_i$. The ZFS change is estimated as the following [3]:

$$D(T) - D(T_0) = \frac{\delta f}{2} \frac{(I_1 + I_2) - (I_3 + I_4)}{(I_1 - I_2) - (I_3 - I_4)}. \tag{S.1}$$

In this case, the reference temperature $T_0$ should be chosen so that $I_1 + I_2$ and $I_3 + I_4$ are equal.

# Fitting method

The fitting method, which is also widely used, estimates the resonance frequencies $f_\pm$ by fitting the ODMR spectrum with a double Lorentzian function and deduces the ZFS as follows,

$$D(T) = \frac{f_+ + f_-}{2}. \tag{S.2}$$

In contrast to the 4-point method, the reference temperature can be set arbitrarily with the fitting method.

# Gaussian process regression (GPR)

In this study, we use GPR, a nonparametric machine learning protocol commonly applied to function estimation [4, 5, 6], to determine temperature. GPR can estimate the function $y = f(\boldsymbol{x})$ from the input variable $\boldsymbol{x}$ and the output variable $y$. We use the ODMR spectra as input variables and the temperatures corresponding to the spectra as output variables. In other words, a function $f(\boldsymbol{x})$ is obtained to estimate a temperature from a given spectrum $\boldsymbol{x}$. The GPR method learns the relationship between the spectral shape and the corresponding temperature. GPR is characterized by the kernel function $k(\boldsymbol{x}, \boldsymbol{x}')$, which represents the degree of coincidence of the two input variables $\boldsymbol{x}$, $\boldsymbol{x}'$. We use the squared exponential kernel, a generally used kernel function, given as follows:

$$k(\boldsymbol{x}, \boldsymbol{x}') = \exp(-\theta ||\boldsymbol{x} - \boldsymbol{x}'||^2). \tag{S.3}$$

As training data, $n$ input variable vectors $\boldsymbol{x}_i$ and output scalar variables $y_i$ are prepared. Assuming that the input variable is $\boldsymbol{x}'$, the estimated output value $f(\boldsymbol{x}')$ is as follows:

$$f(\boldsymbol{x}') = \boldsymbol{k}(\boldsymbol{x}')^{\mathrm{T}} (K + \beta^{-1} I)^{-1} \boldsymbol{y}, \tag{S.4}$$

where $I$ is an identity matrix, $\boldsymbol{y}$ is a column vector with $y_i$ as its $i$-th entry, $\boldsymbol{k}(\boldsymbol{x}')$ is a column vector with $k(\boldsymbol{x}_i, \boldsymbol{x}')$ as its $i$-th entry, $K$ is an $n \times n$ matrix with $K_{ij} = k(\boldsymbol{x}_i, \boldsymbol{x}_j)$ as its $(i, j)$-th entry, and $\beta^{-1}$ is the noise intensity on the output variable $y$. In the present work, $\boldsymbol{x}_i$ is the ODMR spectrum,

and $y_i$ is the true temperature. There are only two hyperparameters: the variable $\theta$ and the noise of acquired data $\beta^{-1}$. For robust analysis, we normalize the contrast of the ODMR spectrum and use the data after the first derivative with respect to frequency as input variables [2]. When $N_p$ is smaller than 321 points, the analysis is first performed by extracting $N_p$ data points from the raw spectrum of 321 points. Therefore, the first derivative is performed only after extracting $N_p$ data.

We comment on the essential differences and similarities between the GPR and conventional methods. In the GPR method, the information of the entire ODMR spectrum is used to estimate temperature, and the assumption of temperature dependence of the ZFS [7], Eq. (1) in the main text, is unnecessary. The selection of the frequency points for measurement or analysis is also arbitrary. However, training data is required to use the GPR method. It is similar to the need to calibrate ZFS at the reference temperature $D(T_0)$ and coefficient $\alpha$ in the conventional methods.

# Evaluation of estimation accuracy

We explain how to evaluate the estimation accuracy of the three methods using the two ODMR spectrum data sets (#1 and #2) at each temperature. First, in the 4-point method, the temperatures are initially estimated based on the 4-point method formula (Eq. (S.1)) using Data #1. The reference temperature is set at 280 K. The reference temperature is then redefined to minimize the RMSE between the estimated and true temperatures in Data #1. The proportionality coefficient $\alpha$ in Eq. (1) in the main text is determined from the relationship between the ZFS calculated by the 4-point method formula and the corresponding temperature. Using the redefined reference temperature and the coefficient $\alpha$, we deduce the temperatures with Data #2. Second, in the fitting method, Data #1 is used to obtain $\alpha$ in Eq. (1) in the main text by fitting the ODMR spectrum with a double Lorentzian. Based on Eq. (1) in the main text, the temperature is estimated from the ZFS obtained by fitting the spectrum of Data #2. Third, the GPR method uses Data #1 to learn the relationship between the ODMR spectra and the corresponding temperatures. This learning result is used to estimate temperature from Data #2. In this way, we use Data #1 as calibration data for the 4-point and fitting methods and training data for the GPR method. Data #2 is used as test data to obtain RMSE.

# References


[1] Kensuke Ogawa, Moeta Tsukamoto, Kento Sasaki, and Kensuke Kobayashi. Lock-in thermography using diamond quantum sensors. *Journal of the Physical Society of Japan*, 92(1):014002, 2023.

[2] Moeta Tsukamoto, Shuji Ito, Kensuke Ogawa, Yuto Ashida, Kento Sasaki, and Kensuke Kobayashi. Accurate magnetic field imaging using nanodiamond quantum sensors enhanced by machine learning. *Scientific Reports*, 12(1):13942, 2022.

[3] Masazumi Fujiwara, Alexander Dohms, Ken Suto, Yushi Nishimura, Keisuke Oshimi, Yoshio Teki, Kai Cai, Oliver Benson, and Yutaka Shikano. Real-time estimation of the optically detected magnetic resonance shift in diamond quantum thermometry toward biological applications. *Physical Review Research*, 2(4):043415, 2020.

[4] David JC MacKay. Introduction to gaussian processes. *NATO ASI Series F Computer and Systems Sciences*, 168:133–166, 1998.

[5] Carl Edward Rasmussen and Christopher K. I. Williams. *Gaussian processes for machine learning*, volume 2. MIT press Cambridge, MA, 2006.

[6] Yukito Iba and Shotaro Akaho. Gaussian process regression with measurement error. *IEICE TRANSACTIONS on Information and Systems*, 93(10):2680–2689, 2010.

[7] M. C. Cambria, G. Thiering, A. Norambuena, H. T. Dinani, A. Gardill, I. Kemeny, V. Lordi, Á. Gali, J. R. Maze, and S. Kolkowitz. Physically motivated analytical expression for the temperature dependence of the zero-field splitting of the nitrogen-vacancy center in diamond. *Physical Review B*, 108(18):L180102, 2023.
